# Supplementary material for: FIND: A Function Description Benchmark for Evaluating Interpretability Methods
Source: arXiv:2309.03886 source file (2023-12-08)
Supplement: Supplementary file 1 [file 00_titleauthor_appendix.tex]

\title{FIND: A Function Interpretation Benchmark for Evaluating Interpretability Methods \\ Appendix}

\author{%
% Sarah Schwettmann$^{1}$\thanks{Indicates equal contribution. Address correspondence to: schwett@mit.edu, tamarott@mit.edu} \quad Tamar Rott Shaham$^{1}$\footnotemark[1] \quad Joanna Materzynska$^1$ \\ \textbf{Neil Chowdhury}$^1$ 
% \quad \textbf{Shuang Li}$^1$ \quad 
% \textbf{Jacob Andreas}$^1$ \quad \textbf{David Bau}$^2$ \quad \textbf{Antonio Torralba}$^1$\\
% \\
% $^1$MIT CSAIL \quad $^2$Northeastern University\\
}
